# Supplementary material for: TRCF: Temporal-Reference Complementary Forecasting for Irregular Multivariate Time Series
Source: arXiv:2611.26351 source file (2026-11-19)
Supplement: Supplementary file 1 [file appendix_experiments.tex]

\section{Additional experimental evidence}
\label{app:experiments}
\suppressfloats[t]
This appendix provides the full protocols and supporting experiments for
the four questions in Section~\ref{sec:experiments}. Core comparison
tables remain in the main text; the analyses below retain the additional
controls, diagnostics, and sensitivity results.

\subsection{Evaluation and training protocol}
\label{app:protocol}
\label{sec:evaluation}
\paragraph{Data and evaluation.}
We use HumanActivity (HA), USHCN, PhysioNet P12, and MIMIC-III, with
12, 5, 36, and 96 variables,
respectively~\citep{vidulin2010activity,debrouwer2019gruode,silva2012challenge,johnson2016mimic}.
HA forecasts 0.3 seconds from three seconds of history. USHCN forecasts
the next three retained timestamp rows after approximately three years
of a four-year station record. MIMIC uses half-hour bins through
35.5 hours and forecasts the next three retained timestamp rows.
P12 averages repeated measurements within their actual hourly bins,
uses history strictly before hour 36, and forecasts the first three
occupied bins thereafter. Its 36 retained channels and standardization
statistics are fitted on the training cohort; measurements with absolute
standardized value at least five are masked. General admission
descriptors are excluded from the dynamic variables.

The inherited train/validation/test proportions are 81/9/10\%.
HA is split by activity record before window extraction. USHCN uses
the first seeded split of benchmark records; MIMIC uses an ordered
split of benchmark record identifiers. The test splits
contain 218/112/1,199/2,125 samples and
5,910/368/27,008/23,015 scored targets for TRCF, in dataset order.
The official PrimeNet and tPatchGNN collators retain 26,828 targets on
P12 and 18,057 on MIMIC; the other evaluated models score 27,008 and
23,015 targets, respectively.
MSE and MAE pool errors over the retained observed future targets, including the
incomplete final batch. Both metrics use the same selected checkpoint.
The reported repetitions characterize optimization variation on fixed
cohorts; sample standard deviations for our runs use denominator $n-1$
for $n$ seeds. Published HA/USHCN baseline deviations are retained as reported.
The controlled signal study uses three seeds (2024--2026).

\paragraph{Comparisons.}
We retain APN's complete published external baseline list in
Table~\ref{tab:main-results}: PrimeNet, NeuralFlows, CRU, mTAN, SeFT,
GNeuralFlow, GRU-D, Raindrop, Warpformer, tPatchGNN, and
GraFITi~\citep{liu2026apn}. Their HA and USHCN entries use the
published means and standard deviations. On P12 and MIMIC, the eleven
baselines and APN use the official APN repository implementations and
training, validation, early-stopping, and test procedures, with five
seeds (2024--2028). P12 data interfaces read the existing prepared
records. MIMIC uses the original benchmark fold~0 and its cached
normalization through the native data loader. These runs retain
model-specific losses, batch sizes, learning rates, epoch limits,
checkpoint selection, and batch construction, including the target-count
exceptions above. The prepared records and partitions agree with those
used by KAFNet and TRCF. KAFNet uses its
official implementation, the released HA launcher settings and the
entry-point defaults for the other datasets, without additional
hyperparameter search~\citep{zhou2026kafnet}. Its native training loss is
retained, while checkpoint selection uses complete-validation point MSE.
The quantitative comparisons with APN and KAFNet below refer to these
shared-input evaluations.

\paragraph{Training and controls.}
TRCF uses $K=16$ temporal slots, $G=32$ grid cells, width-16
directional TCNs, one four-head variable-attention layer, and
$\mathcal L_{\mathrm{MSE}}+0.1\mathcal L_{\mathrm{hist}}$.
Adam runs for at most 200 epochs with patience ten. The direct learning
rate is unchanged for three epochs, then multiplied by 0.8 after each
subsequent epoch; auxiliary parameters use one tenth of that rate.
Training retains the native shuffled, drop-last loader. TRCF checkpoints
minimize complete-validation point MSE; ties retain the latest epoch.
Table~\ref{tab:configuration} lists dataset-specific settings.
\input{tables/current_configuration}

The real-data component and sensitivity studies retain this forecast objective,
checkpoint rule, data stream, and paired seeds. A removal changes its
specified computation; an alternative changes its stated representation.
Historical reconstruction uses weight 0.1 unless a comparison explicitly
varies or omits that objective. The main configuration is
held fixed throughout these studies. TRCF, component studies, and the
P12 and MIMIC official baseline runs use an RTX 5090 GPU.


\paragraph{Complete benchmark comparisons.}
TRCF lowers mean MSE and MAE relative to APN on all four datasets.
MSE decreases by 3.44\%, 10.06\%, 2.54\%, and 6.47\% on
HA, USHCN, P12, and MIMIC, respectively; MAE decreases by
3.09\%, 3.38\%, 2.60\%, and 4.12\%.
The corresponding MSE reductions against the evaluated KAFNet
configurations are 2.55\%, 25.32\%, 3.08\%, and 9.60\%;
MAE also decreases on all four datasets. These comparisons use
forecast MSE as TRCF's sole future-target objective.

Both errors improve against APN in all five seed pairs on HA, P12,
and MIMIC. USHCN improves in three of five pairs and has a wider
optimization spread, despite its larger mean gain. Against the evaluated
KAFNet configurations, both errors decrease in all five pairs on each
dataset. The KAFNet result characterizes the stated configurations under
our task setting, rather than its performance under additional tuning.

\paragraph{Clinical baseline comparison.}
On MIMIC, TRCF has the lowest five-seed mean MSE and MAE among
the evaluated models. Relative to Warpformer, the strongest other mean
for both metrics, MSE decreases by 5.73\% and MAE by 3.16\%; both
metrics improve in all five paired seeds.
On P12, TRCF's mean MSE and MAE are 0.04\% and 0.42\% lower than
GraFITi's, respectively. The MSE difference is smaller than either
model's seed standard deviation, so this mean ranking does not establish
a clear advantage over GraFITi.
\paragraph{Inference-memory profiling.}
We profile the main-table APN and TRCF configurations on the same
RTX 5090 in FP32 eager execution. Each pair receives the same first
three full validation batches, with batch sizes shown in
Table~\ref{tab:inference-memory}. We use the seed-2024 checkpoints,
evaluation mode, and \texttt{inference\_mode}. After 20 warm-up calls,
we measure 100 calls per batch and report the largest PyTorch allocated
memory peak across the three batches. The measurement includes the model,
input batch, and prepared TRCF factor cache; one-time cache construction
and data transfer are outside the measured region. Test MSE uses the five-seed means of the same model configurations.

TRCF reduces measured peak inference memory relative to APN by
87.98\%, 71.55\%, 17.28\%, and 67.02\% on HA, USHCN, P12,
and MIMIC, respectively, while lowering mean test MSE.
Table~\ref{tab:inference-resources} shows that this memory advantage
coexists with more model parameters. The result concerns the evaluated
batch shapes and original model configurations; it does not isolate
the memory contribution of an individual module.

\input{tables/inference_resources_full}

\subsection{Parameter allocation and context controls}
\label{app:capacity}
\begingroup
\let\TRCFsavedtable\table
\renewcommand{\table}[1][]{\TRCFsavedtable[H]}
\input{tables/context_parameters}
\input{tables/encoder_context}
\endgroup

\paragraph{Matched direct encoders.}
Table~\ref{tab:matched-slot-budget} compares direct predictors using
adaptive patches at the original dataset-specific budget or at $P=16$,
and ANCHOR at $K=16$. All share the forecast objective, checkpoint
rule, feature width, time embedding, token processing, and prediction
interface. Reducing the adaptive encoder to 16 patches does not recover
ANCHOR's accuracy: ANCHOR lowers mean MSE by 3.02\%, 14.80\%,
1.36\%, and 0.77\% on HA, USHCN, P12, and MIMIC, respectively,
and lowers mean MAE on all four datasets. Both errors improve in all
five pairs on the first three datasets; MIMIC MSE improves in three
pairs and MAE in all five.


ANCHOR also retains fewer parameters at the same slot count. On
MIMIC, the complete direct predictor uses 4,113 parameters, compared
with 7,249 for 16 adaptive patches, a 43.26\% reduction. The corresponding
reduction on HA is 1.47\%, where the shared processing layers dominate.
Thus slot count alone does not explain the observed test-accuracy difference,
while the size advantage depends on the dataset configuration. The
USHCN ordering is cohort-sensitive: ANCHOR has 7.26\% higher
selected-validation MSE than the 16-patch encoder, despite its lower
test MSE.

Adaptive patch geometry contains $2NP+N$ learned parameters for
positions, widths, and variable temperatures; ANCHOR learns $K$
shared widths with fixed centers. These counts concern pooling geometry,
whereas the table counts the complete predictors. The matched-slot-count
comparison still changes geometry, sharing, and support representation
together. It does not assign the gain to Gaussian kernels or fixed centers
alone. Appendix~\ref{app:anchor-details} examines individual ANCHOR choices.

\paragraph{Encoder--context interaction.}

We combine each direct encoder with the same BRIDGE module.
Table~\ref{tab:encoder-context} gives the resulting two-by-two
comparison under the common forecast loss and checkpoint rule.


Table~\ref{tab:encoder-context} evaluates BRIDGE relative to each
encoder alone. On MIMIC, BRIDGE lowers MSE by 4.52\% with adaptive
patches and by 4.25\% with ANCHOR; corresponding MAE reductions are
2.76\% and 2.63\%. Its benefit therefore extends to both temporal
encoders. The complete models have nearly equal MIMIC MSE, with
0.40407 for adaptive patches plus BRIDGE and 0.40428 for TRCF.

USHCN shows a different interaction. BRIDGE lowers MSE by 1.67\%
with adaptive patches but raises it by 4.77\% with ANCHOR; MAE rises
by 0.69\% and 1.04\%, respectively. The MSE reversal shows that
context cannot be judged independently of the direct representation
it supplements. On HA and P12, BRIDGE's MSE gains are smaller with
ANCHOR than with adaptive patches. Together, these comparisons locate
the principal USHCN improvement in the compact encoding configuration
and the principal MIMIC improvement in BRIDGE context.


\paragraph{Matched-capacity constructions and training.}
The encoder--context comparison changes representation, capacity, and historical supervision together. We use three controls. \emph{Widened ANCHOR} reallocates the entire context-branch budget to the direct token FFN. \emph{Interpolated context} linearly fills the shared grid, extends the nearest observation at boundaries, and uses zero for unsupported variables. \emph{Temporal context} retains bidirectional temporal estimates but removes residual propagation and cross-variable correction. Both context controls retain ANCHOR, the variable encoder, fusion scale, and prediction head, while preserving observed grid values.

The context controls reallocate removed parameters to their variable-encoder FFN. Added widths follow analytic parameter counts, rounded upward to meet or exceed the full-model parameter count without validation tuning. Common weights are copied at initialization, and additional FFN units have zero outgoing weights.

TRCF and temporal context use $\lambda_h\in\{0,0.1\}$, while interpolated context and widened ANCHOR use $\lambda_h=0$. For temporal context, the two-term historical objective supervises directional estimates and their mean before observations are restored. Zero-weight comparisons evaluate construction without historical supervision. All settings use five paired seeds, the same data streams, forecast MSE, validation-MSE checkpoint rule, and the corresponding branch learning rates. They share the epoch limit and early-stopping rule; realized epoch and update counts can differ.





Tables~\ref{tab:context-parameters} and~\ref{tab:context-capacity} separate parameter allocation from context construction. With $\lambda_h=0$, TRCF reduces MIMIC MSE by 5.29\% relative to widened ANCHOR, 4.27\% relative to interpolated context, and 3.33\% relative to temporal context; all five seeds improve in both MSE and MAE for each comparison. On P12, the corresponding MSE reductions are 0.95\%, 0.64\%, and 0.45\%, again in all five seeds, although MAE differences are smaller. Interpolated and temporal context also improve mean MSE over widened ANCHOR on both datasets. These results support allocating capacity to a historical representation and show an additional benefit from the full construction beyond these two simpler alternatives.

This construction advantage remains when both TRCF and temporal context use $\lambda_h=0.1$: MSE falls by 3.24\% on MIMIC and 0.38\% on P12, with the same direction in all five seeds. It therefore does not depend on assigning historical supervision only to the full model. Widening the direct FFN alone does not reproduce the clinical MSE gains.

The effect is not universal. On Human Activity, interpolated context has the lowest mean MSE, and the differences among context variants are small. On USHCN, ANCHOR retains the lowest mean MSE, while widened ANCHOR has the lowest mean MAE. TRCF has lower selected-validation MSE than temporal context at both historical-loss weights but higher test MSE; the corresponding P12 and MIMIC comparisons retain their validation direction on the test set. Thus the USHCN reversal cannot be generalized to the two clinical datasets, nor can the clinical gains justify adding context everywhere.

On the two clinical test sets, historical reconstruction exhibits an MSE--MAE trade-off in the full model. Raising $\lambda_h$ from 0 to 0.1 increases full-model MSE by 0.31\% on P12 and 0.68\% on MIMIC, despite reducing mean MAE; temporal context likewise has higher MSE at 0.1 on these datasets. The clinical MSE advantage of the full construction is already present without this auxiliary objective. Together, these controls support a conditional role for constructed context, rather than extra parameters or historical reconstruction as a universal explanation of improvement.

\subsection{Message-construction controls}
\label{app:message-controls}
% Integrate with the complete attribution results, never partial seed outcomes.
\paragraph{Reference construction versus source availability.}
We cross reference-relative and raw-value completion with nearest-source
and observed-only availability. Let $b\in\{0,1\}$ choose the reference:
observed messages are $X-b\mu$, and the completion adds $b\mu$ to the
correction. Nearest-source lookup, exact-tie averaging, distance decay,
target exclusion, loading geometry, and the output-offset convention
are identical between the two reference conditions. Observed-only
availability sets missing-cell source weights to zero. The direct
encoder, variable encoder, fusion, initialization, and training recipe
remain paired across all four conditions.

The raw controls retain both directional temporal-reconstruction terms
and the completion loss with the same historical weight. Their temporal
estimator is trained but does not enter raw completion or forecasting.
The comparison therefore tests using a learned reference in source
construction and reconstruction together; it does not isolate the
subtraction operation alone or compare separately tuned model families.
The reference effect is measured within each availability condition,
and the propagation effect within each reference condition.


\paragraph{Reference choice does not uniformly improve error.}
Under nearest-source availability, reference-relative completion lowers
HA MSE by 0.08\% but raises USHCN, P12, and MIMIC MSE by 0.24\%,
0.51\%, and 0.36\% relative to the raw control. Its mean MAE is lower
on HA, P12, and MIMIC, but higher on USHCN. On MIMIC, residual and
raw completion obtain MSE/MAE of 0.40428/0.38160 and
0.40283/0.38372, respectively: using the reference raises MSE in four
of five pairs while lowering MAE in four. On P12, raw nearest-source
completion has lower MSE in every pair. These controls do not support
attributing the forecasting gain uniquely to reference-relative messages;
the reference changes the balance between the two test-error metrics.
Selected-validation MSE favors the reference on P12 and MIMIC by
0.25\% and 0.84\%, respectively, reversing the test ordering.
The observed test-error trade-off therefore does not establish an
intrinsic MSE--MAE trade-off of reference-relative communication.

\paragraph{Source availability has a distinct effect.}
On MIMIC, nearest-source propagation lowers MSE relative to observed-only
availability with both residual messages (1.85\%) and raw messages
(1.59\%). MSE decreases in all five pairs for both constructions;
mean MAE also decreases by 0.80\% and 0.39\%, respectively.
The propagation effect is much smaller on HA and P12, and neither
construction benefits in mean USHCN error. Figure~\ref{fig:attribution-effects}
separates this availability effect from reference choice. Together with
the direct-only comparison, the MIMIC results give stronger evidence
for access to nearby cross-variable sources than for universal
superiority of residual messages.

\begin{figure}[t]
\centering\includegraphics[width=\linewidth]{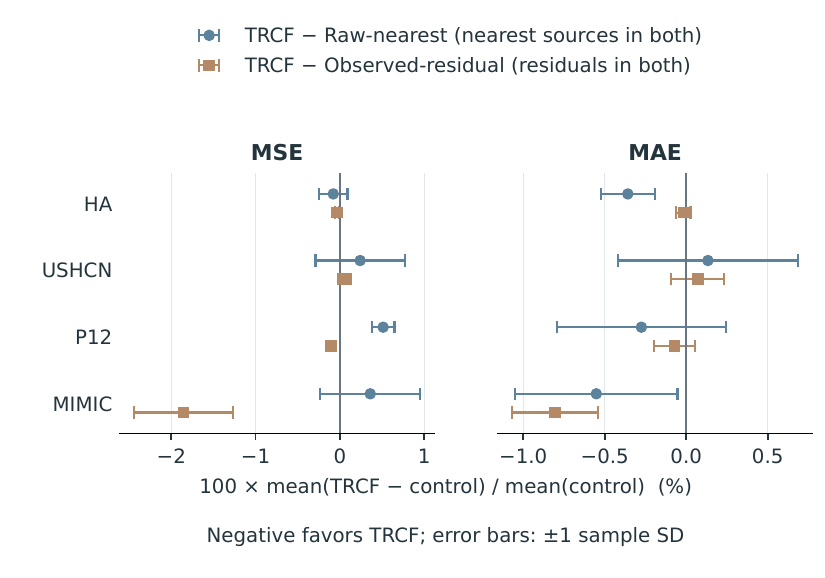}
\caption{Reference and source-availability contrasts over five paired seeds. Points show relative error change, and error bars show the sample standard deviation of paired differences divided by the control mean. The plot names both comparisons explicitly; negative values favor TRCF.}
\label{fig:attribution-effects}
\end{figure}


\input{tables/bridge_mechanisms}
\paragraph{Which parts of message construction help?}
Within BRIDGE, removing cross-variable correction sets $\Delta=0$.
Temporal completion and the variable encoder remain, so this comparison
tests residual correction beyond temporal estimates and variable
attention. Removing residual relay permits source contributions only
at observed grid cells, testing access to asynchronous source residuals.
On MIMIC, these removals raise MSE/MAE by 3.52\%/2.16\% and
1.89\%/0.81\%, respectively. Both metrics worsen in every seed pair
for both controls. Residual correction and access to nearby source
deviations therefore contribute to forecasting in this setting.

\paragraph{Model-filled raw values as an alternative.}
\input{tables/completion_alternative}
A separate raw-value alternative uses observed values at measured source cells
and channel-local estimates at missing source cells. Its regressor
predicts values directly, including its bias, instead of adding a
residual correction to the target reference. This changes the source
construction and the reconstruction rule together. On MIMIC it raises
MSE/MAE by 1.03\%/1.28\%, with both errors higher in all five pairs.
It compares two complete context-building strategies; the separate
propagation and correction removals provide the more targeted mechanism
evidence. On USHCN, all three internal alternatives produce small
changes relative to the complete model, whereas deleting BRIDGE
improves both metrics.

\subsection{Controlled signal dependence and sampling conditions}
\label{app:controlled-signals}
\label{sec:controlled-conditions}
We separate three factors: shared versus independent deviations,
persistent versus rapidly changing deviations, and synchronous versus
asynchronous sampling. Each of the eight regimes uses eight variables,
768 training records, 192 validation records, and 256 test records.
A trajectory is the sum of a variable-specific smooth sinusoidal
background, an Ornstein--Uhlenbeck deviation, and measurement noise
with standard deviation 0.05. Deviations have standard deviation 0.5
and time constant 0.15 or 0.01 over a unit historical interval. Shared
deviations combine a common process with alternating signed loadings
of magnitude 0.8 and independent components; independent deviations
retain the same marginal variance without the common component.

Writing the generated deviation as
$\eta_n(t)=a_n z(t)+\sqrt{1-a_n^2}\,u_n(t)$, with independent
stationary processes of variance $v=0.25$ and common time constant
$\tau$, gives
\begin{equation}
 \operatorname{Cov}(\eta_n(t),\eta_j(s))
 =v a_n a_j\exp(-|t-s|/\tau),\qquad n\ne j.
 \label{eq:controlled-covariance}
\end{equation}
Here $a_n=\pm0.8$ in the shared condition and zero otherwise.
This relation specifies how sharing, persistence, and source distance
change the available latent association. Its incremental forecasting
value also depends on what the target's own history already reveals.

Every variable has exactly 16 observations among 257 historical time
points. Synchronous sampling uses the same locations for every variable;
asynchronous sampling circularly shifts those locations independently
for each variable. Values are sampled at their actual times. The dense
trajectory and three future targets remain identical across sampling
conditions; query times are $(264,272,280)/256$.
This manipulation also changes grid occupancy and gaps to
the history endpoint, which we measure alongside coincidence.

We compare ANCHOR alone, TRCF, raw nearest-source completion, and
residual observed-only completion with three paired optimization seeds.
All use width 16, time-embedding width 8, $K=16$, and no dropout;
the context variants use $G=32$ and $\beta=0.1$.
Training uses Adam with initial direct rate $10^{-3}$,
a cosine schedule to $10^{-4}$ over 100 epochs, auxiliary-rate multiplier
0.1, batch size 64, and patience 15. Checkpoints minimize complete
validation MSE. Generator seeds are independent of optimization seeds.
Latent trajectories are excluded from model inputs and training labels;
validation diagnostics compare the learned reference with the known
background and residuals with the generated deviations at observed
historical grid cells, after aggregating the known components with the
same grid rule. These
diagnostics describe the learned decomposition, while future-target
errors test its forecasting value.

\input{tables/controlled_conditions}
\begin{figure}[t]
\centering\includegraphics[width=\linewidth]{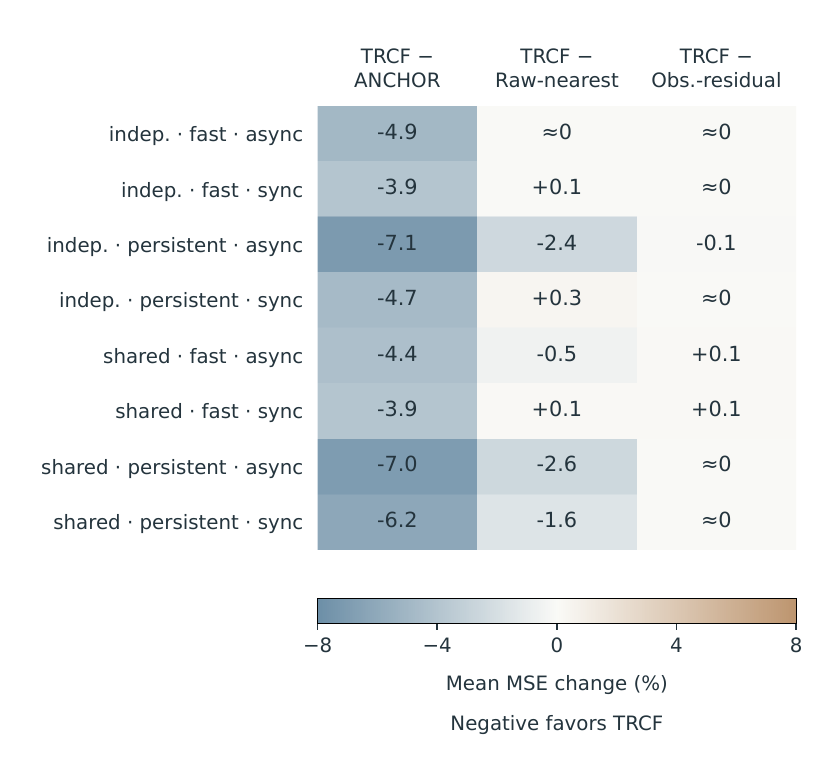}
\caption{Controlled-signal test MSE changes over three paired seeds, relative to each column control. All columns use the same zero-centered scale. Labels with absolute change below $0.05\%$ are shown as $\approx0$; other labels are rounded to one decimal place. This threshold denotes display precision, not significance. Negative values favor TRCF; full test results are in Table~\ref{tab:controlled-conditions}.}
\label{fig:controlled-conditions}
\end{figure}

\paragraph{Branch gains and message effects differ.}
TRCF lowers MSE by 3.88--7.10\% and MAE by 1.74--3.71\%
relative to ANCHOR across the eight regimes, with both errors lower
in all three seed pairs in each regime.
The improvements also occur with independent deviations.
The direct predictor has 2,305 parameters and each context variant
has 8,388. Adding the branch changes capacity, temporal reconstruction,
historical representation, and training objective together; its total gain
therefore does not identify the use of shared cross-variable deviations.

The targeted propagation contrast is much smaller.
Replacing observed-only residual sources with nearest sources changes
MSE by $-0.073$\% to $+0.097$\% and MAE by $-0.048$\% to
$+0.039$\%. Mean MSE slightly increases in all four shared regimes.
Thus these controlled forecasts do not reproduce the material relay
benefit seen on MIMIC, or support the proposed explanation that shared,
persistent deviations make residual relay consistently beneficial.
The reference comparison has a different pattern: with persistent
asynchronous signals, reference-relative construction lowers MSE
against raw nearest-source completion by 2.44\% for independent
deviations and 2.56\% for shared deviations, with both metrics improving
in all three pairs. The benefit in both cases again separates this
effect from a requirement for shared deviations.
Under independent persistent synchronous signals, however, the
reference raises MSE by 0.32\%. Its relative effect is more favorable
under asynchronous sampling in each of the four signal conditions,
but the selected-validation MSE favors references in all eight regimes
and three synchronous regimes reverse that ordering on test.

\paragraph{Signal manipulation and learned references.}
The validation diagnostics confirm distinct latent conditions.
At a lag of $8/256$, generated deviation correlations are
0.803--0.807 for persistent signals and 0.041--0.043 for fast signals.
Mean absolute cross-variable correlations are 0.628--0.635 under
sharing and 0.005--0.018 under independence. Asynchronous sampling
reduces exact-time coincidence from 1 to 0.062, with grid coverage
0.407 versus 0.410 and mean endpoint gap 0.055 versus 0.064.
The sampling comparison therefore changes several aspects of
available history even though each variable retains 16 observations.

The learned decomposition also differs from the known generating
components. For TRCF, the three-seed mean correlation between observed
residuals and generated deviations is 0.578--0.588 in persistent
regimes, versus 0.804--0.809 in fast regimes. Reference MSE relative
to the generated background is 0.158--0.167 and 0.115--0.117,
respectively. The background serves as a diagnostic component and is
not assumed to be the reconstruction-optimal temporal reference:
persistent deviations themselves contain predictable history.
These diagnostics do not justify applying the known latent covariance
in Eq.~\ref{eq:controlled-covariance} directly to the learned residual
messages; their cross-variable covariance is not measured here.
Together, the controlled comparisons locate the explanatory gap
between improving a complete historical-context branch and showing
that its nearest-source residual mechanism provides the improvement.

\subsection{Historical support and reconstruction diagnostics}
\label{app:diagnostics}
\label{sec:conditional-diagnostics}
We stratify the unchanged evaluation histories by grid coverage,
non-coincidence of observed variables, and source gaps on the 32-cell
history grid. The source-gap score averages, over target-missing cells
and other variables, the distance to each source variable's nearest
observation, normalized by the grid span. Unobserved sources receive
a score of one, combining missing availability with temporal distance. Tercile boundaries use
training histories only and retain ties. Within each nonempty stratum,
we pool target errors and compare the same five fitted seeds.
Intervals use 2,000 bootstrap draws after averaging error sums across
seeds. HA windows are grouped by their source activity record; each
held-out split contains only three such records. Other datasets use
their benchmark record units. These intervals describe variation
conditional on the fitted models and observed records, with limited
resolution for HA. Support strata describe associations and do not
identify causal effects of missingness or asynchrony.

A separate validation-only reconstruction diagnostic hides
$\min(\lceil0.2n\rceil,n-2)$ grid cells in a channel with $n\geq3$
observed cells. The hidden mask is shared across models and
seeds. Grid coordinates remain fixed, hidden values are removed, and
temporal gaps are recomputed before predicting those values. We measure
temporal-reference and completed-history errors and the correlation of
nearest remaining within-channel deviations and cross-variable corrections
with held-out
deviations. This tests historical message quality separately from
future forecasting accuracy.

\paragraph{Support conditions and forecasting.}
On the original MIMIC test split, adding BRIDGE to ANCHOR changes
MSE by $-4.25\%$, with a 95\% record-bootstrap interval of
$[-5.46,-2.97]\%$. Its change is $-6.92\%$ in the low-coverage
stratum and $-0.88\%$ in the high-coverage stratum; the latter interval
includes zero. USHCN has the opposite pattern: the branch raises test
MSE by 14.60\% under low coverage, 13.46\% under high grid
non-coincidence, and 13.44\% under large source gaps. Sparse or
non-coincident histories therefore do not uniformly favor this context.

Even within MIMIC, the non-coincidence trend depends on the split.
Across low, middle, and high strata, the branch changes test MSE by
$-3.51\%$, $-4.06\%$, and $-5.23\%$, respectively; the corresponding
validation changes are $-6.11\%$, $-4.12\%$, and $-2.50\%$.
This reversal limits a general explanation based on increasing asynchrony.
The original USHCN cohorts also differ in error concentration: the two
records with the largest five-seed mean full-model squared-error sums,
ranked separately within each split, account for
68.91\% of validation error, compared with 14.29\% of test error.
This identifies a difference in error distribution, without establishing
the cause of the validation--test ordering reversals.

\paragraph{Historical reconstruction and future prediction.}
For full TRCF, completed histories have lower hidden-cell MSE than their temporal
references by 23.43\%, 3.11\%, 20.08\%, and 19.75\% on
HA, USHCN, P12, and MIMIC. This evaluates reconstruction at known
grid coordinates, rather than unseen future times. The propagation
contrast is smaller: relative to the model using only observed residual
sources, the full model's reconstruction MSE is 0.37\% higher on USHCN
and 0.08\% lower on MIMIC. Thus improvement over a temporal reference
does not by itself identify a propagation benefit, and the historical
reconstruction ordering is not interchangeable with the forecasting
ordering. These diagnostics support evaluating the representation and
its contribution to the final predictor separately.

\subsection{Primary path removals}
\label{app:internal-ablation}
\label{sec:ablation}
\paragraph{Architectural dependence.}
The two removals in Table~\ref{tab:module-ablation} examine how
the complete predictor uses its two paths. Removing ANCHOR deletes
the direct slots, query pooling, and associated normalization. BRIDGE,
its original fusion coefficient, zero-initialized output projection,
auxiliary learning rate, and the future-time prediction head remain.
Removing BRIDGE leaves the direct path and removes historical
reconstruction. These are path removals under the full model's training
recipe. In particular, the context-only variant retains the optimization
settings of an auxiliary branch.
\input{tables/module_ablation}
\input{sections/new_module_results}

\begin{figure}[H]
\centering\includegraphics[width=\linewidth]{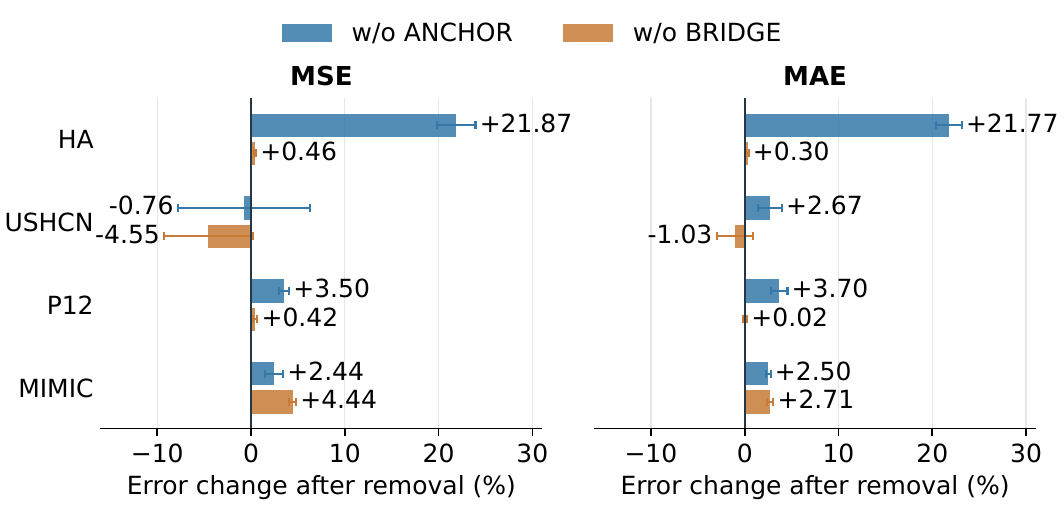}
\caption{Error change after removing each path. Positive values mean removal hurts; negative values mean removal helps. Bars are five-seed mean paired changes normalized by the full-model mean; error bars show one sample standard deviation of paired changes.}
\label{fig:module-effects}
\end{figure}
Figure~\ref{fig:module-effects} separates the two removal effects while retaining the USHCN reversal.

\subsection{ANCHOR geometry, support, and observation retention}
\label{app:anchor-details}
\begin{figure}[H]
\centering\includegraphics[width=\linewidth]{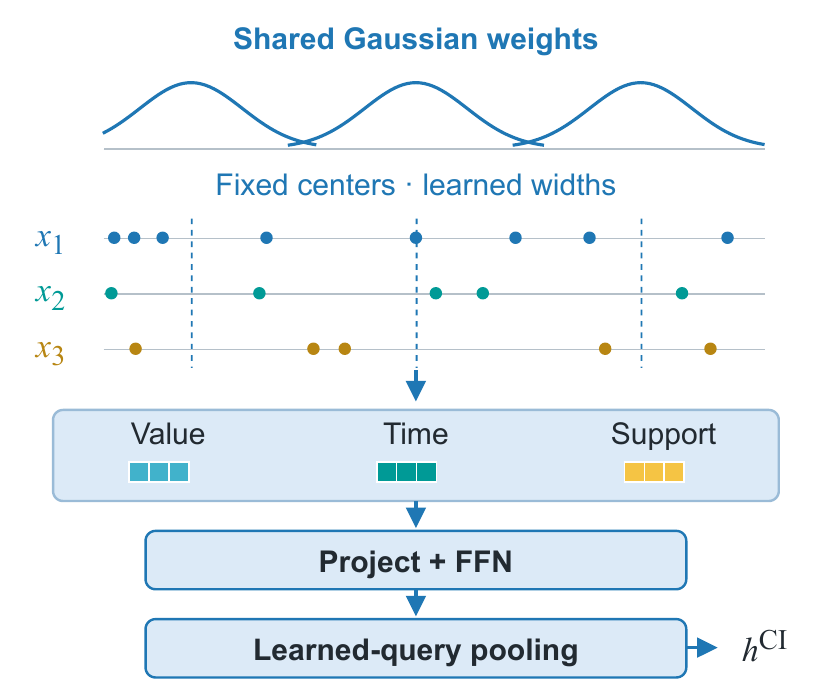}
\caption{ANCHOR representation construction. The top row shows Gaussian aggregation weights separately from the observed value--time inputs below. Shared centers and learned widths define temporal slots; each variable aggregates its own measurements and support. Projection, token processing, and learned-query pooling produce the direct representation. Curves and token counts are schematic; the main model uses $K=16$.}
\label{fig:anchor-mechanism}
\end{figure}
\label{sec:anchor-factors}
Three matched alternatives
isolate the aggregation choices: learn
unconstrained shared centers from the same initial positions; remove the support
feature while retaining the projection dimensions; and learn independent
widths for each variable from identical initial widths. Kernel shape,
slot count, time embedding, token processing, and BRIDGE are unchanged.
The learned-center and independent-width variants give identical initial
predictions to the full model.
We also use a fixed 0.1 learning-rate multiplier for center parameters
alone, retaining all other learning rates and the same scheduler.
This control examines whether the center comparison depends on its
update scale; it uses the same multiplier on every dataset.
\IfFileExists{sections/new_anchor_results.tex}{\input{sections/new_anchor_results}}{}

\paragraph{Observation support and center adaptation.}
On USHCN and MIMIC, we retrain the fixed- and learned-center models at
nominal history retention rates of 25\%, 50\%, and 100\%. Deterministic
nested masks are shared across all three variants and all optimization
seeds in training, validation, and test. For a variable with $n>0$
observations, a rate $r$ retains $\lceil rn\rceil$ entries; actual
retention can therefore exceed the nominal rate. The 25\%/50\% schedules
retain 25.69\%/50.49\% of USHCN test observations and
40.63\%/58.88\% of MIMIC test observations. Only historical values
and masks change. Future queries, target values, and scoring masks
remain unchanged. This experiment tests learning under reduced support.
We also record fitted center displacement as a descriptive diagnostic;
movement alone does not establish that adaptation is harmful.
\IfFileExists{sections/new_retention_results.tex}{\input{sections/new_retention_results}}{}

\subsection{Parameter sensitivity and model width}
\label{app:sensitivity}
\label{sec:sensitivity}
We next examine resolution and fusion parameters: $K$
controls temporal compression in ANCHOR, $G$ controls the alignment
resolution in BRIDGE, and $\beta$ scales its projected features before fusion.
We vary one parameter at a time on USHCN and MIMIC, using
$K\in\{8,16,32\}$, $G\in\{16,32,64\}$, and
$\beta\in\{0.05,0.1,0.2\}$. Figure~\ref{fig:sensitivity} shows
validation changes around the frozen default.
\begin{figure}[t]
\centering\includegraphics[width=\linewidth]{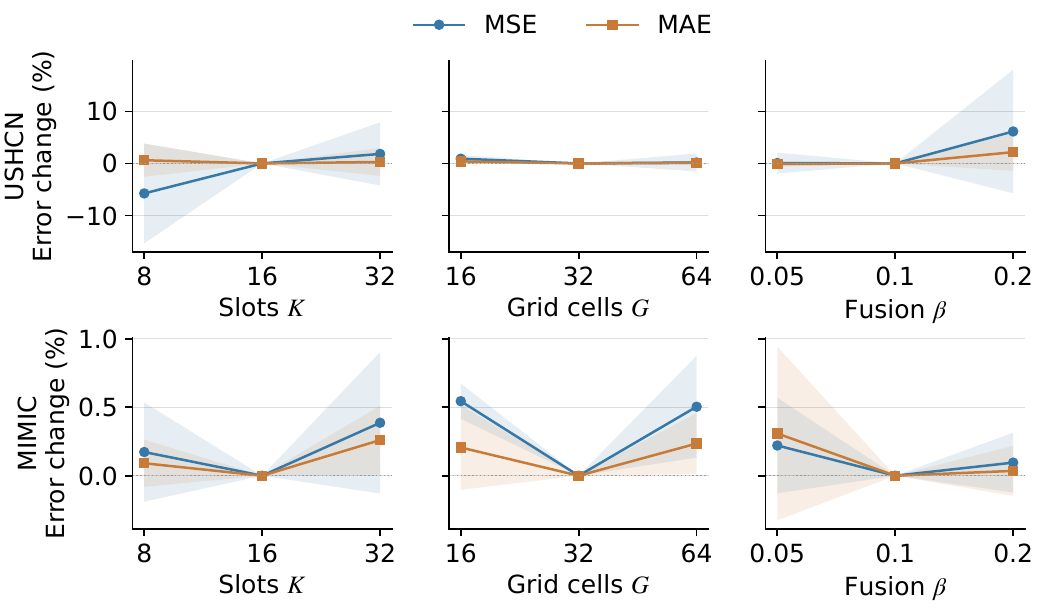}
\caption{Validation sensitivity on two datasets, five paired seeds.
For seed $s$, the change is $100(e_s-e_{0,s})/\bar e_0$, where
$e_{0,s}$ is the default error. Lines show means and bands one sample
standard deviation. The reference is zero by definition; rows use
different vertical scales. Positive values indicate higher error.}
\label{fig:sensitivity}
\end{figure}
MIMIC mean MSE varies by at most 0.55\% and mean MAE by at most 0.31\%
over these settings. USHCN is more sensitive: $K=8$ lowers validation
MSE by 5.75\%, whereas $\beta=0.2$ raises it by 6.14\%.
The corresponding $K=8$ test MSE rises by 7.08\%, showing that the
validation preference does not transfer uniformly to the fixed test
cohort. We retain the original main setting rather than selecting a
configuration from test performance.

\paragraph{Width and parameter count.}
The full model has 36,292/6,843/12,164/19,332 parameters on
HA/USHCN/P12/MIMIC. The larger HA count follows its inherited direct
width $D=56$, compared with $6/24/16$ on the other datasets.
Its slot FFN alone has 12,712 parameters. KAFNet has 5,135 parameters
in the evaluated HA configuration and 65,775 on each other dataset;
its model widths are 16 and 64, respectively. Parameter counts therefore
reflect the evaluated configurations, including their different widths.
\IfFileExists{sections/new_width_results.tex}{\input{sections/new_width_results}}{}

\subsection{Secondary components and training objectives}
\label{app:training-objective}
\label{sec:loss-ablation}
\input{tables/secondary_components}
Replacing off-diagonal variable attention with diagonal attention has
small, mixed effects: on MIMIC, MSE increases by 0.15\% while MAE
falls by 0.10\%. Setting $\lambda_h=0$ lowers MIMIC MSE by 0.68\%
but raises MAE by 0.10\%. On this MIMIC configuration, these changes have smaller MSE effects than
the correction and propagation removals. The corresponding effects remain
specific to the compared training recipes and operators.

A separate five-seed loss comparison adds $0.1\mathcal L_{\mathrm{MAE}}$
to the forecasting objective while leaving the model and historical
loss unchanged. Test MAE improves on all four datasets, but test MSE
improves only on USHCN. The main model uses no forecast MAE term,
so the gains in Table~\ref{tab:main-results} do not depend on that addition.
\input{tables/forecast_loss_ablation}

\subsection{Additional partition protocol and complete comparisons}
\label{app:partition-protocol}
We repeat the principal comparisons on USHCN and MIMIC using two
additional random record partitions, fixed with seeds 31001 and 31002,
and three optimization seeds per partition. The same benchmark records
are assigned approximately 81/9/10\% to training, validation, and test.
For each partition, channel means and population standard deviations
are fitted only to observed historical values in its training records,
then applied to every split. Time scales use fixed nominal horizons.
The future-query rule, model configurations, optimization budget,
checkpoint selection, and target masks remain paired across methods.

For MIMIC, we recover physical measurement values before fitting the
new normalization. USHCN starts from the supplied benchmark values;
its upstream processing is retained. Earlier filtering and binning are
inherited in both datasets, and no new clipping or record exclusion is
introduced. This study changes both partition and normalization relative
to the original prepared-input evaluation, so its scores are reported
separately. It tests repeatability within the benchmark's record units,
not generalization to an external cohort.


On MIMIC, BRIDGE lowers test MSE relative to ANCHOR by 3.63\%
and 3.90\% in the two additional partitions, with lower MSE and MAE
in all three paired seeds in each partition. Residual propagation also
improves over observed residuals in both partitions: MSE decreases by
1.57\% and 1.14\%, again in all three pairs. These results retain the
context and source-availability effects under the two additional
partition-and-normalization settings.

Message content has a different pattern. Raw-value propagation retains
lower mean MSE than residual propagation on MIMIC in both partitions.
The residual construction lowers MAE by 0.88\% in partition 31001,
but raises it by 0.09\% in partition 31002. Thus the original
MSE--MAE ordering is not a stable advantage of either construction
across evaluation cohorts.

USHCN is more sensitive to the partition. Adding BRIDGE raises mean
MSE by 1.93\% in partition 31001 and lowers it by 3.63\% in
partition 31002. ANCHOR lowers mean test MSE relative to 16 adaptive
patches in all four dataset--partition cells, while using fewer parameters;
only two of three paired seeds agree in each cell, and its USHCN MAE
is higher in partition 31002. Against the original-budget adaptive encoder,
ANCHOR's USHCN MSE changes by $-8.70\%$ and $+3.95\%$ across
the two partitions. In the latter partition, its selected-validation MSE
is 2.28\% lower despite the higher test MSE. Compact encoding remains
competitive, but neither its accuracy nor the value of context has a
uniform ordering across these records.
